# Supplementary material for: Verifying Lock-free Search Structure Templates
Source: arXiv:2405.13271 source file (2024-05-22)
Supplement: Supplementary file 1 [file appendix.pdf]

## 948 **A** Proof of Traversals

949 We provide additional details on the proof of the eager traversal, as well as the implementation  
950 and proof of the lazy traversal.

### 951 **A.1** Proof of Eager Traversal

952 We describe the proof of `eager_i` in more detail. Let us formally define the traversal invariant  
953 `EagerInv` for `eager_i` as follows:

$$954 \quad \text{EagerInv}(k, p, c) := \Diamond(\text{mark}(p, 0) = \text{false} \wedge \text{key}(p) < k) * \Diamond(k \in \text{inset}(c))$$

955 The predicate `EagerInv` captures the fact that `eager_i` witnessed node  $p$  to be unmarked and  
956 its key less than  $k$  at some point during its traversal. Additionally, it witnessed that  $k$  was  
957 in the inset of  $c$  at some prior state of the structure. We put the two facts about  $p$  and  $c$  in  
958 separate  $\Diamond$  predicates because the two facts may hold for different past states.

```

1  {EagerInv(k, p, c)}
2  let eager_i 0 k p c =
3    match findNext 0 c with
4    | cn, true ->
5      match changeNext 0 p c cn with
6      | Success ->
7        {EagerInv(k, p, c) * mark(p, 0) = false * next(p, 0) = cn * key(p) < k}
8        {mark(p, 0) = false * key(p) < k * k ∈ inset(p) * k ∈ outset(p) * k ∈ inset(cn)}
9        {EagerInv(k, p, cn)}
10       eager_i 0 k p cn
11     | Failure -> traverse ps cs k
12   | cn, false ->
13     {EagerInv(k, p, c) * mark(c, 0) = false * next(c, 0) = cn}
14     {EagerInv(k, p, c) * mark(c, 0) = false * next(c, 0) = cn
15       * (key(c) < k ⇒ k ∈ EagerInv(k, c, cn))
16       * (k ≤ key(c) ⇒ ◇(k ∈ keyset(c)))}
17   let kc = getKey c in
18   if kc < k then
19     {EagerInv(k, c, cn)}
20     eager_i 0 k c cn
21   else
22     {◇(k ∈ keyset(c))}
23     let res = (kc = k ? true : false) in
24     (p, c, res)
25     {◇(k ∈ keyset(c) ∧ res ⇔ k ∈ C(c))}

```

■ **Figure 12** Outline for the proof of the `eager_i` for the base level.

959 For the moment, assume that predicate `EagerInv`( $k, p, c$ ) holds at the beginning of the  
960 function call `eager_i 0 k p c`. The proof outline in Figure 12 shows that this is sufficient to  
961 prove the `traverse` specification. We explain the critical steps of the proof in the following.

962 The first critical step occurs when  $c$  is found to be marked, and the subsequent `changeNext`  
963 call on  $p$  succeeds (Line 6). Immediately after this step, we can establish that `mark`( $p, 0$ ) =  
964 `false` and `next`( $p, 0$ ) =  $cn$  due to the success of `changeNext`. The Invariant 3 allows us to  
965 infer `key`( $p$ ) <  $k$  from `EagerInv`( $k, p, c$ ). In addition, we use the following structural invariant:

966 **Invariant 5** For all nodes  $n$ , if  $\text{mark}(n, 0)$  is set to *false* then  $[\text{key}(n), \infty) \subseteq \text{inset}(n)$ . As a  
 967 consequence of the definition of edgesets and  $\text{outset}(n)$  (from Section 3.1), we additionally  
 968 obtain  $\text{outset}(n) = (\text{key}(n), \infty)$ .

969 Invariant 5 helps us establish that  $k \in \text{inset}(p)$ ,  $k \in \text{outset}(p)$  and since  $\text{next}(p, 0) = cn$ ,  
 970 also  $k \in \text{inset}(cn)$ . Using the rule that  $q$  implies  $\Diamond q$  for an arbitrary proposition  $q$ , we can  
 971 establish  $\text{EagerInv}(k, p, cn)$  before the recursive call on Line 10.

972 The second critical step is when  $\text{findNext}$  determines  $c$  to be unmarked (Line 12). The  
 973 proof goes by case analysis, depending on whether  $\text{key}(c) < k$  holds. First consider that this  
 974 condition is true. Similar to the first critical step, we are able to establish  $\text{EagerInv}(k, c, cn)$   
 975 here as we have all the relevant facts at this moment. The predicate  $\text{EagerInv}(k, c, cn)$  is  
 976 used for the recursive call on Line 18. Now consider the case that  $k \leq \text{key}(c)$ . Here, we  
 977 use  $\Diamond(k \in \text{inset}(c))$  provided by  $\text{EagerInv}(k, p, c)$ . Let  $t$  be the time point when  $k \in \text{inset}(c)$   
 978 held true. Since  $c$  is unmarked currently,  $c$  must also have been unmarked at time  $t$  due  
 979 to Invariant 2. And by Invariant 5, we can establish that  $k \notin \text{outset}(c)$  at time  $t$ . Thus, we  
 980 conclude that also  $k \in \text{keyset}(c)$  held at time  $t$ . Similarly we conclude that  $C(c) = \{\text{key}(c)\}$   
 981 as  $c$  is unmarked. Putting this all together, we obtain:

$$982 \quad k \in C(c) \iff k = \text{key}(c) \iff \text{res.}$$

983 This concludes the proof that predicate  $\text{EagerInv}$  is indeed an invariant for  $\text{eager\_i}$  and is  
 984 sufficient to prove the  $\text{traverse}$  specification.

985 In the previous proof, we assumed  $\text{EagerInv}$  holds when  $\text{eager\_i}$  begins executing at the  
 986 base level. The final piece remaining from the complete proof of the  $\text{traverse}$  specification  
 987 is to show that  $\text{eager\_i}$  collects enough information at higher levels to establish  $\text{EagerInv}$   
 988 before traversing the base level. We explain this below.

989 It is easy to see that for all higher levels  $i$ ,  $\text{eager\_i}$  can establish  $\Diamond(\text{mark}(p, i) = \text{false} \wedge$   
 990  $\text{key}(p) < k)$  when it returns  $(p, \_, \_)$ . (In fact,  $\text{EagerInv}$  contains the exact same facts about  
 991  $p$  and the same argument as in the proof outline for the base level is applicable.) Thus,  
 992 when a predecessor  $p$  is chose from the higher level to initiate  $\text{eager\_i}$  at the base level, we  
 993 know that  $\Diamond(\text{mark}(p, i) = \text{false} \wedge \text{key}(p) < k)$  holds. The current node  $c$  is chosen by calling  
 994  $\text{findNext } 0 \ p$  at Line 16 in Figure 4. If  $\text{findNext}$  determines  $p$  to be unmarked, then we can  
 995 establish  $k \in \text{inset}(c)$  using the fact  $\Diamond(\text{key}(p) < k)$  and Invariant 5. However, if  $p$  is found to  
 996 be marked, then it is a bit tricky to establish that  $\Diamond(k \in \text{inset}(c))$ . We require the following  
 997 additional structural invariant.

998 **Invariant 6** For all nodes  $n$ , if there exists an  $i$  such that  $\text{mark}(n, i)$  is set to *false*, then  
 999  $\text{mark}(n, 0)$  is set to *false*.

1000 Invariant 6 captures the fact that the base level gets marked at the end. This fact is useful  
 1001 for us because we can combine it with  $\Diamond(\text{mark}(p, i) = \text{false})$  to obtain  $\Diamond(\text{mark}(p, 0) = \text{false})$ .  
 1002 Since  $\text{findNext}$  has found  $p$  to be marked at the base level, we can determine that it got  
 1003 marked at some time point between the point in time when  $\Diamond(\text{mark}(p, 0) = \text{false})$  held and  
 1004 the present. Let  $t$  be the time point right before  $p$  got marked. The following invariant gives  
 1005 us useful information about which node  $\text{next}(p, 0)$  can be pointing to at time  $t$ :

1006 **Invariant 7** For all nodes  $n$  and level  $i$ , once  $\text{mark}(n, i)$  is set to *true*,  $\text{next}(n, i)$  does not  
 1007 change.

1008 Invariant 7 preceisely says that  $\text{next}(p, 0) = c$  at time  $t$ . Thus, we have found a moment  
 1009 in time when  $\text{mark}(p) = \text{false}$ ,  $\text{key}(p) < k$  and  $\text{next}(p, 0) = c$ . These three facts allow us  
 1010 to immediately conclude that  $k \in \text{inset}(c)$  at time  $t$ . This finally completes the proof of  
 1011  $\text{traverse}$ .

## 1012 A.2 Lazy Traverse

1013 The code for the lazy traversal is shown in Figure 13. While the `lazy_rec` implementation is  
 1014 almost identical to `eager_rec`, the two differ in the per-level traversal in `lazy_i` and `eager_i`.  
 1015 The `lazy_i` function here keeps track of three nodes while traversing: node  $p$  is the last  
 1016 unmarked node it witnessed, node  $pn$  is the node that  $p$  was pointing to when  $p$  was traversed,  
 1017 and  $c$  is the node that is currently being traversed. The function `lazy_i` begins by reading  
 1018 the next pointer and mark bit of  $c$ . If  $c$  is found to be marked, then `lazy_i` simply continues  
 1019 with the successor of  $c$ . If  $c$  is unmarked, then the operation key  $k$  is compared with `key(c)`.  
 1020 In case `key(c) < k`, then again `lazy_i` continues with  $c$  as the last seen unmarked node.  
 1021 Otherwise,  $k \leq \text{key}(c)$ . In this case, it attempts to unlink the marked segment between  
 1022 nodes  $p$  and  $c$ . The conditional on Line 10 checks if there is a segment to remove. If that is  
 1023 indeed the case, then `lazy_i` calls `changeNext` to unlink the segment between  $p$  and  $c$ . If  
 1024 `changeNext` succeeds, then there is a further check to make sure  $c$  is still unmarked. If so,  
 1025 then `lazy_i` returns with  $p$  and  $c$ . In all other cases where `changeNext` fails or  $c$  is found to  
 1026 be marked, `lazy_i` restarts the `traverse` function.

```

1  let lazy_i i k p pn c =
2  match findNext i c with
3  | cn, true -> lazy_i i k p pn cn
4  | cn, false ->
5    let kc = getKey c in
6    if kc < k then
7      lazy_i i k c cn cn
8    else
9      let res = (kc = k ? true : false) in
10     if pn = c then
11       (p, c, res)
12     else
13       match changeNext i p pn c with
14       | Success ->
15         let _, b = findNext i c in
16         if b then traverse ps cs k
17         else (p, c, res)
18       | Failure -> traverse ps cs k
19
19 let lazy_rec i ps cs k =
20   let p = ps[i+1] in
21   let c, _ = findNext i p in
22   let p', c', res = lazy_i i k p c c in
23   ps[i] <- p';
24   cs[i] <- c';
25   if i = 0 then
26     (p', c', res)
27   else
28     lazy_rec (i-1) ps cs k
29
30 let traverse ps cs k =
31   lazy_rec (L - 2) ps cs k

```

■ **Figure 13** The lazy traversal for the skiplist template corresponding to the Harris List style traversal.

## 1027 A.3 Proof of Lazy Traversal

1028 The proof idea for the lazy traversal is similar to that of the eager traversal. We provide a  
 1029 brief overview of the traversal invariant for `lazy_i`, and why it is sufficient to establish the  
 1030 required specification for `traverse`. The following discussion focuses on the `lazy_i` executing  
 1031 on the base level, for sake of simplicity.

1032 The traversal invariant for `lazy_i` is defined as below:

$$\begin{aligned}
 \text{LazyInv}(k, p, pn, c) &:= \text{EagerInv}(k, p, pn) * (pn \neq c \Rightarrow \exists ls. \text{MarkedSeg}(pn, ls, c)) \\
 \text{MarkedSeg}(pn, ls, c) &:= (ls = [] \Rightarrow \Diamond(\text{next}(pn, i) = c)) \\
 &\quad * (ls = [n_0, \dots, n_l] \Rightarrow \Diamond(\text{next}(pn, 0) = n_0) \\
 &\quad \quad * (\forall 0 \leq j < l. \Diamond \text{next}(n_j, 0) = n_{j+1})) \\
 &\quad * \Diamond(\text{next}(n_l, 0) = c)
 \end{aligned}$$

The invariant `LazyInv` relies on `EagerInv` and a new predicate `MarkedSeg` that stores the segment of marked nodes. Additionally, the predicate establishes that the nodes  $pn$  and  $c$  are the start and end points of the marked segment.

To see that `LazyInv` is indeed an invariant, consider Lines 3 and 7 where `lazy_i` is recursively called. At Line 3, the marked segment can be extended by including the marked node  $c$ , while  $p$  and  $pn$  remain unchanged. On the other hand, at Line 7, the second conjunct of `LazyInv` becomes trivially true, and  $eagerinv(k, c, cn)$  can be established in the same way as for `eager_i`.

Let us now show why `LazyInv` is sufficient to prove the `traverse` specification. Consider the points where `lazy_i` terminates (lines 11 and 17). When terminating at Line 11, we know that  $pn = c$ . Hence, `LazyInv` provides the predicate `EagerInv(k, p, c)`. Using the same argument as `eager_i`, we can establish the required postcondition. Now consider Line 17. In this case, the thread has successfully unlinked the marked segment, hence it can establish that  $mark(p, 0) = false$  and  $next(p, 0) = c$  right after the call to `changeNext`. Note that the later check whether  $c$  is unmarked must succeed in order for `lazy_i` to terminate. Hence, at the point of the successful `changeNext`,  $c$  must also be unmarked, giving us all the facts necessary to establish the required postcondition. This completes the proof of `lazy_i`.

## B Soundness of Hindsight Specification

This section focuses on the soundness of the Hindsight specification, i.e., the proof that any structure that satisfies (`HindSpec`) must also satisfy (`ClientSpec`). We begin with some background on Iris that will be necessary for the proof, followed by additional details on the predicate `Hist` and the helping invariant  $Inv_{help}$ . Finally, we provide a proof outline relating (`HindSpec`) to the (`ClientSpec`).

### B.1 Iris Primer

Iris is a state-based concurrent separation logic. Assertions in the logic express ownership of resources. These resources include both physical resources that are manipulated by the program as well as ghost resources that capture auxiliary information for the purpose of the proof and that are manipulated using the proof rules of the logic. An example of an assertion describing a physical resource is the points-to predicate,  $\ell \mapsto v$ , which expresses ownership of heap location  $\ell$  and constrains its stored value to be  $v$ . Two assertions  $P$  and  $Q$  (e.g. describing disjoint heap regions) can be composed using a *separating conjunction*,  $P * Q$ . The logic supports standard local reasoning principles such as the *frame rule*: if the Hoare triple  $\{P\} e \{Q\}$  is valid, then so is  $\{P * R\} e \{Q * R\}$  for all *frames*  $R$ .

To describe ghost resources, Iris provides assertions of the form  $\llbracket a \rrbracket^\gamma$  which state ownership of a chunk  $a$  of the ghost resource stored at ghost location  $\gamma$ . The chunk  $a$  must be drawn from a *camera* that is specified as part of the proof. Cameras generalize the partial commutative monoids that are commonly used to define the semantics of separating conjunction. The precise definition of these structures is immaterial for this paper. What is important is that a camera is a set  $S$  equipped with an operation  $a \cdot b$  that is compatible with separating conjunction in the following way:  $\llbracket a \rrbracket^\gamma * \llbracket b \rrbracket^\gamma \dashv\vdash \llbracket a \cdot b \rrbracket^\gamma$ . A simple example is the `MaxNat` camera defined by  $S = \{\text{Max}(n) \mid n \in \mathbb{N}\}$  and  $\text{Max}(n) \cdot \text{Max}(m) = \text{Max}(\max(n, m))$ .

A proof can introduce ghost resources as needed by allocating a fresh ghost location  $\gamma$ . A proof can also update chunks of ghost resources at existing ghost locations using *view shifts*,  $\llbracket a \rrbracket^\gamma \Rightarrow \llbracket b \rrbracket^\gamma$ . A view shift is only allowed if replacing  $a$  by  $b$  is *frame-preserving*. Intuitively, this means that for any  $c$  such that the full ghost resource stored at  $\gamma$  may be  $a \cdot c$  before the

1083 update,  $b$  must also compose with  $c$ . For example, in the **MaxNat** camera, all updates are  
 1084 frame-preserving because composition (maximum) is totally defined. However, in general,  
 1085 this is not the case.

1086 To reduce the burden on the proof author, Iris provides a library of predefined parameter-  
 1087 ized cameras. One such camera that we will use below is the *agreement camera*  $\text{Ag}(X)$  which  
 1088 is defined for any set  $X$ . The elements take the form  $\text{agree}(x)$  for  $x \in X$  and composition is  
 1089 only defined in the case of identity:  $\text{agree}(x) \cdot \text{agree}(x) = \text{agree}(x)$ . Another predefined camera  
 1090 we will use is that of finite partial maps from some set  $X$  to some camera  $R$ ,  $\text{Map}(X, R)$ ,  
 1091 with composition defined by lifting the composition on  $R$  pointwise to maps.

1092 To enable reasoning about shared resources, Iris provides the notion of an *invariant*. Any  
 1093 Iris assertion  $P$  can be turned into an invariant, denoted  $\boxed{P}$ . Once an invariant has been  
 1094 created, it becomes a duplicable resource, which means that it can be commonly owned by  
 1095 all threads. An individual thread may access (and manipulate) the resources described by  
 1096 the underlying assertion  $P$  when performing a computation step, provided  $P$  is reestablished  
 1097 after each step.

A reoccurring pattern in Iris proofs is to have an invariant that holds authoritative  
 ownership of the current state of a resource, and each thread may additionally own partial  
 knowledge about this resource that the thread gathered during its execution. To encode  
 this pattern, Iris provides the *authoritative camera*  $\text{Auth}(R)$  defined over any camera  $R$ . The  
 authoritative camera has elements of the form  $\bullet a$  to denote authoritative ownership of  
 $a \in R$  and  $\circ a$  to denote *fragmental* ownership. The composition  $\bullet a \cdot \circ b$  expresses the fact  
 that  $b$  is a fragment of  $a$ , i.e.,  $\exists c, a = b \cdot c$ . For example, the camera  $\text{Auth}(\text{MaxNat})$  is very  
 useful to establish lower bounds of a monotonically non-decreasing quantity. The definitions  
 of  $\text{Auth}(\text{MaxNat})$  yields the valid entailment:  $\boxed{\bullet \text{Max}(n)} \multimap \boxed{\bullet \text{Max}(n')} \multimap \boxed{\circ \text{Max}(n')}$ . The  
 permitted frame-preserving updates are shown below:

$$\begin{array}{c} \text{AUTH-MAX-UPD} \frac{n \leq n'}{\boxed{\bullet \text{Max}(n)} \multimap \boxed{\bullet \text{Max}(n')}} \\ \text{AUTH-MAX-SNAP} \boxed{\bullet \text{Max}(n)} \multimap \boxed{\bullet \text{Max}(n)} \multimap \boxed{\circ \text{Max}(n)} \end{array}$$

1098 The rule **AUTH-MAX-UPD** requires that the update only increases the authoritative value to  
 1099 guarantee that the new authoritative value  $n'$  still composes with all fragmental values.

## 1100 B.2 Tracking the Computation History

1101 Hindsight arguments involve reasoning about past program states. Our encoding therefore  
 1102 tracks information about past states using *computation histories*. We define computation  
 1103 histories as finite partial maps from *timestamps*,  $\mathbb{N}$ , to *snapshots*,  $\mathbb{S}$ . A snapshot describes an  
 1104 abstract view of a program state at a particular time. It is a parameter of our encoding. For  
 1105 instance, a snapshot may capture the physical memory representation of the data structure  
 1106 under proof, while abstracting from the remainder of the program state. Another parameter  
 1107 of our encoding is a function  $|\cdot|$  that computes the abstract state of the data structure from  
 1108 a given snapshot.

1109 The predicate  $\text{Hist}(H, T)$  consists of two ghost resources: one resource to store the  
 1110 authoritative computation history  $H$ , and one resource to store the last timestamp  $T$  used in  
 1111  $H$ . Whenever the program changes the program state in a way that is observable at the level  
 1112 of snapshots, the invariant forces  $H$  to be updated with a new snapshot at time  $T + 1$ , and  $T$   
 1113 to be increased by 1. To track  $T$ , we use the camera  $\text{Auth}(\text{MaxNat})$ , which implicitly encodes

the fact that timestamps are non-decreasing, effectively serializing the snapshot changes in the history.

We want threads to be able to own fragmental knowledge of the authoritative history  $H$ . These history fragments are then used to define past predicates that express the existence of a past state with a certain snapshot. To this end, we use the camera  $\text{Auth}(\text{Map}(\mathbb{N}, \text{Ag}(\mathbb{S})))$  for the resource that tracks the history. The use of the agreement camera ensures that the history can only be updated by appending to it (i.e., all snapshots of past states are preserved).

The predicate  $\text{Hist}(H, T)$  is then defined as

$$\text{Hist}(H, T) := \left[ \bullet \text{Max}(T) \right]^{\gamma_t} * \left[ \bullet \text{agree}(H) \right]^{\gamma_m} \\ * \text{dom}(H) = \{0 \dots T\} * \forall t < T. H(t) \neq H(t+1) .$$

Here, we abuse notation and write  $\text{agree}(H)$  for the function that takes the history  $H$  to an element of  $\text{Auth}(\text{Map}(\mathbb{N}, \text{Ag}(\mathbb{S})))$  in the expected way. The second last conjunct ensures that the authoritative history contains no gaps. The purpose of the last conjunct is to ensure that a thread appends to the history whenever any change to the program state is made that affects the snapshot (see discussion in Section 4.2).

### B.3 Augmenting $\text{op}$ with Prophecies

In light of the discussion in Section 4.1, we must augment  $\text{op}$  with auxiliary ghost code that creates and resolves the relevant prophecies. We do this by defining the wrapper function  $\overline{\text{op}}$  given in Figure 14. Let us first briefly discuss how prophecy variables can be used in Iris. The right side of Figure 14 shows the specifications of the two functions related to manipulating prophecies. The function  $\text{NewProph}$  returns a fresh prophecy  $p$  that predicts a sequence of values  $pvs$ , captured by the resource  $\text{Proph}(p, pvs)$ . This resource can be owned and shared among threads via a shared invariant. The resource is also non-duplicable.

The values contained in the sequence  $pvs$  are determined by how  $p$  is resolved using the  $\text{Resolve}$  command. The rule  $\text{PROPHECY-RESOLUTION}$  ties the observed value ( $v$ ) to the next prophesied value (the head of  $pvs$ ). It also updates  $\text{Proph}(p, pvs)$  to the tail of  $pvs$  for the remaining prophesied values that are yet to be observed. In our context, we want the prophecy to predict whether the decisive operations (i.e.  $\text{markNode}$  and  $\text{changeNext}$ ) will succeed as well as their return value. Hence, we augment  $\text{delete}$  and  $\text{insert}$  by wrapping their decisive operations inside a  $\text{Resolve}$  command. The return value is captured by the resolution on Line 5. For our purposes, we assume that  $pvs$  is a sequence of  $\text{Success}$  or  $\text{Failure}$  values (i.e., the result of each attempted call to the decisive operation) followed by a special value  $\text{END}(res)$  indicating that no further future calls are expected, and that  $res$  will be the final return value<sup>2</sup>. Given the prophesied sequence of values  $pvs$ , a thread will exhibit an unmodifying linearization point iff  $pvs$  does not contain any  $\text{Success}$  values.

Let us now turn to  $\overline{\text{op}}$ , which starts by generating a unique thread identifier using  $\text{NewThreadID}$  on Line 2. We also implement  $\text{NewThreadID}$  using the  $\text{NewProph}$  construct. There are two benefits to this: (i) Iris makes sure that prophecy identifiers are unique out of the box, and (ii) now we can use Iris's erasure theorem for prophecies to argue that the augmented code  $\overline{\text{op}}$  has the same behavior as  $\text{op}$ . After,  $\overline{\text{op}}$  creates a prophecy  $p$  as described

<sup>2</sup> We have to also consider the case where  $pvs$  is not of this form, but that is a trivial case to handle and thus we do not consider it in this discussion.

|                                                     |                                                                                                                           |
|-----------------------------------------------------|---------------------------------------------------------------------------------------------------------------------------|
| 1 <b>let</b> $\overline{\text{op}}$ $r$ $k$ =       | PROPHECY-CREATION                                                                                                         |
| 2 <b>let</b> $tid$ = NewThreadID <b>in</b>          | $\{\text{True}\} \text{NewProph } \{p. \exists pvs. \text{Proph}(p, pvs)\}$                                               |
| 3 <b>let</b> $p$ = NewProph <b>in</b>               |                                                                                                                           |
| 4 <b>let</b> $v$ = $\text{op } p \ r \ k$ <b>in</b> | PROPHECY-RESOLUTION                                                                                                       |
| 5 Resolve $p$ to $\text{END}(v)$ ; $v$              | $\{\text{Proph}(p, pvs)\} \text{Resolve } p \text{ to } v$<br>$\{\exists pvs'. \text{Proph}(p, pvs') * pvs = v :: pvs'\}$ |

■ **Figure 14** Wrapper augmenting  $\text{op}$  with prophecy-related ghost code, whose specification is given on the right.

$$\begin{aligned}
\boxed{\text{Inv}(r)} &:= \exists H T C. \overline{\text{CSS}}(r, C) * |H(T)| = C \\
&\quad * \text{Hist}(H, T) * \text{Inv}_{\text{help}}(H, T) * \text{Inv}_{\text{tpl}}(H, T) \\
\text{Inv}_{\text{help}}(H, T) &:= \exists R. \left[ \bullet R \right]^{\gamma_r} \\
&\quad * \bigstar_{tid \in R} \exists \text{op } k v_p t_0 \Phi \text{Tok}. \text{Reg}(tid, \text{op}, k, v_p, t_0, \Phi, \text{Tok}) \\
\text{Reg}(tid, \text{op}, k, v_p, t_0, \Phi, \text{Tok}) &:= \text{Thread}(tid, t_0) * \boxed{\text{State}(\text{op}, k, v_p, t_0, \Phi, \text{Tok})} \\
\text{State}(\text{op}, k, v_p, t_0, \Phi, \text{Tok}) &:= \text{Pending}(\text{op}, k, v_p, t_0, \Phi) \vee \text{Done}(\text{op}, k, v_p, t_0, \Phi, \text{Tok}) \\
\text{Pending}(\text{op}, k, v_p, t_0, \Phi) &:= \text{AU}_{\text{op}}(\Phi) * \neg \text{PastLin}(\text{op}, k, v_p, t_0) \\
\text{Done}(\text{op}, k, v_p, t_0, \Phi, \text{Tok}) &:= (\Phi(v_p) \vee \text{Tok}) * \text{PastLin}(\text{op}, k, v_p, t_0)
\end{aligned}$$

■ **Figure 15** Definition of the invariant encoding the helping protocol.

1155 above, it invokes the underlying operation  $\text{op}$ , and finally, terminates after resolving  $p$  to the  
 1156 result of  $\text{op}$ .

We can now finally present the client-level specification with  $\overline{\text{op}}$ :

$$\boxed{\text{Inv}(r)} \multimap \langle C. \text{CSS}(r, C) \rangle \overline{\text{op}} \ p \ r \ k \ \langle \text{res } C'. \text{CSS}(r, C') * \Psi_{\text{op}}(k, C, C', \text{res}) \rangle.$$

1157 The next section provides details on our choice of  $\text{Inv}(r)$  and the proof of  $\overline{\text{op}}$ .

## 1158 B.4 Proof of $\overline{\text{op}}$

1159 Figure 15 shows a simplified definition of the invariant that encodes the helping protocol<sup>3</sup>. The  
 1160 definitions are implicitly parameterized by a proposition  $\text{Inv}_{\text{tpl}}(r, H, T)$ , which abstracts from  
 1161 the resources needed for proving that a specific structure satisfies the hindsight specification.

1162 The helping protocol predicate  $\text{Inv}_{\text{help}}(H, T)$  contains a *registry*  $\left[ \bullet R \right]^{\gamma_r}$  of thread IDs  
 1163 with unmodifying linearization points that require helping from other concurrent threads.  
 1164 For each thread ID  $tid$  in the registry, the shared state contains  $\text{Thread}(tid, \_)$  along with  
 1165 the state of  $tid$ , which is either **Pending** or **Done**. **Pending** captures an uncommitted atomic  
 1166 triple, and **Done** describes the operation after it has been committed. Note that we use the

<sup>3</sup> For presentation purposes, the proof outline presented here abstracts from some technical details of the actual proof in Iris.



1167 notation  $\text{AU}_{\text{op}}(\Phi)$  to refer to the atomic update token of  $\text{op}$  and write just  $\text{AU}(\phi)$  when  $\text{op}$  is  
 1168 clear.

1169 The proof outline for  $\overline{\text{op}}$  is shown in Figure 16. The proof begins by creating a thread  
 1170 identifier  $tid$  and prophecy  $p$ . As alluded to earlier,  $\text{NewThreadID}$  is also just  $\text{NewProp}$  in  
 1171 disguise, hence we obtain two prophecy resources, one each for  $tid$  and  $p$ . Before we can  
 1172 invoke  $\text{op}$ , we must record the start time of this thread and perform a case split on  $\text{Upd}(pvs)$   
 1173 to determine if this thread requires helping. For this, we open the invariant at Line 7. To  
 1174 record the start time, we give up the resource  $\text{Proph}(tid, \_)$  to gain a duplicable resource  
 1175  $\text{Thread}(tid, T_0)$  in exchange ( $T_0$  is the current timestamp). The exact details of this exchange  
 1176 are not relevant, so we continue with the case split on  $\text{Upd}(pvs)$ . First consider the case that  
 1177  $\text{Upd}(pvs)$  holds. Then, thread  $tid$  does not require helping and the hindsight specification  
 1178 can ensure that  $\text{op}$  linearizes correctly. This is quite straightforward, so we focus on the  
 1179 other case, i.e.  $\text{Upd}(pvs)$  does not hold.

1180 In order to register the thread for helping, we must establish  $\text{PastLin}(\text{op}, k, v_p, T_0)$  or  
 1181 its negation. Here,  $v_p$  is the return value obtained by scanning for the end marker in  $pvs$ .  
 1182 We proceed by first checking if the thread can be linearized at the current timestamp  $T_0$ .  
 1183 If so, then we can safely linearize the thread right away. So let us focus on the more  
 1184 interesting case where we cannot linearize right away (Line 14). Here, the thread registers  
 1185 itself with the helping protocol by updating  $R$  to  $R \cup \{tid\}$  using an update rule for the  
 1186 authoritative set camera (in Line 18). As part of registering for helping, it first establishes  
 1187  $\text{Pending}(\text{op}, k, v_p, T_0, \Phi)$  by transferring its obligation to linearize to the shared state, captured  
 1188 by the update token  $\text{AU}(\Phi)$ . The condition  $\text{PastLin}(\text{op}, k, v_p, T_0)$  follows from the fact that  
 1189  $\Psi_{\text{op}}(k, |H_0(T_0)|, |H_0(T_0)|, v_p)$  does not hold. The thread also creates a fresh non-duplicable  
 1190 token  $\text{Tok}$  that it will later trade in for the receipt  $\Phi(v_p)$ .

1191 We are now at the point of invocation for  $\text{op}$ . Before continuing further, let us briefly  
 1192 switch to the role played by the concurrent thread that must linearize thread  $tid$ . The helping  
 1193 thread must update the structure, and as per the invariant, update the history  $M$  as well  
 1194 as the helping protocol  $\text{Inv}_{\text{help}}(H, T)$ . In particular, while updating the helping protocol, it  
 1195 scans over all threads registered for helping so far, moving them from state  $\text{Pending}$  to state  
 1196  $\text{Done}$  as per the prophesied return value  $v_p$ .

1197 Let us now return to the proof thread  $tid$  at Line 23. As precondition of  $(\text{HindSpec})$ , we  
 1198 give away  $\text{Proph}(p, pvs)$  and obtain the postcondition (Line 24). Simplifying the postcondition  
 1199 of  $(\text{HindSpec})$  for our case  $\neg \text{Upd}(pvs)$ , we obtain the predicate  $\text{PastLin}(\text{op}, k, v_p, T_0)$ . Next,  
 1200 we make a final resolution of the prophecy on Line 26. Since,  $pvs'$  is the suffix of  $pvs$ ,  $\text{END}(v_p)$   
 1201 must also be the final item in  $pvs'$ . After resolution, we obtain  $\text{END}(v_p) = \text{END}(v)$  and by  
 1202 injectivity of the end marker,  $v_p = v$ .

1203 We now have the predicate  $\text{PastLin}(\text{op}, k, v, T_0)$  which we use to obtain the receipt of  
 1204 linearization from the shared invariant. Because  $\text{PastLin}(\text{op}, k, v, T_0)$  holds now, we know  
 1205 thread  $tid$  cannot be in the  $\text{Pending}$  state. Hence, we know that thread  $tid$  must be in the  
 1206  $\text{Done}$  state. Since the thread owns the unique token  $\text{Tok}$ , it trades it in to obtain  $\Phi(v)$ , which  
 1207 lets it complete the proof of its client-level specification.



```

1  $\boxed{\text{Inv}(r)} * \langle C. \text{CSS}(r, C) \rangle$ 
2 let  $\text{op } r \ k =$ 
3    $\{ \text{AU}(\Phi) \}$ 
4   let  $\text{tid} = \text{NewThreadID}$ 
5    $\{ \text{AU}(\Phi) * \text{Proph}(\text{tid}, \_) \}$ 
6   let  $p = \text{NewProp}$  in
7    $\{ \text{AU}(\Phi) * \text{Proph}(\text{tid}, \_) * \text{Proph}(p, \text{pvs}) * \boxed{\text{Inv}(r)} \}$ 
8    $(* \text{ Open invariant } *)$ 
9    $\{ \text{AU}(\Phi) * \text{Thread}(\text{tid}, T_0) * \text{Proph}(p, \text{pvs}) * \overline{\text{CSS}}(r, C_0) * \text{Inv}_{\text{help}}(H_0, T_0) * \dots \}$ 
10   $(* \text{ Case analysis on } \text{Upd}(\text{pvs}) : \text{only showing } \neg \text{Upd}(\text{pvs}) *)$ 
11   $\{ \text{AU}(\Phi) * \text{Thread}(\text{tid}, T_0) * \text{Proph}(p, \text{pvs}) * \overline{\text{CSS}}(r, C_0) * [\bullet R]^{\gamma_r} * \text{tid} \notin R * \dots \}$ 
12   $(* \text{ Let } v_p \text{ such that } \text{pvs} \text{ contains } \text{END}(v_p) *)$ 
13   $(* \text{ Case analysis on } \Psi_{\text{op}}(k, |H_0(T_0)|, |H_0(T_0)|, v_p) : \text{only showing } \neg \Psi_{\text{op}}(|H_0(T_0)|, |H_0(T_0)|, v_p) *)$ 
14   $\{ \text{Thread}(\text{tid}, T_0) * \text{Proph}(p, \text{pvs}) * \overline{\text{CSS}}(r, C_0) * [\bullet R]^{\gamma_r} * \text{tid} \notin R$ 
15     $\{ \dots * \text{AU}(\Phi) * \text{Thread}(\text{tid}, T_0) * \neg \text{PastLin}(\text{op}, k, v_p, T_0) \}$ 
16     $\{ \dots * \text{AU}(\Phi) * \text{Thread}(\text{tid}, T_0) * \text{Pending}(\text{op}, k, v_p, T_0, \Phi) * \text{Tok} \}$ 
17     $\{ \dots * \text{State}(\text{op}, k, v_p, T_0, \Phi, \text{Tok}) * \text{Tok} \}$ 
18   $(* \text{ Ghost update: } [\bullet R]^{\gamma_r} \Rightarrow [\bullet R \cup \{\text{tid}\}]^{\gamma_r} *)$ 
19   $\{ \text{Thread}(\text{tid}, T_0) * \text{Proph}(p, \text{pvs}) * [\circ \{\text{tid}\}]^{\gamma_r} * \text{Tok} * \overline{\text{CSS}}(r, C_0) * [\bullet R \cup \{\text{tid}\}]^{\gamma_r} * \dots \}$ 
20   $\{ \text{Thread}(\text{tid}, T_0) * \text{Proph}(p, \text{pvs}) * [\circ \{\text{tid}\}]^{\gamma_r} * \text{Tok} * \overline{\text{CSS}}(r, C_0) * \text{Inv}_{\text{help}}(H_0, T_0) * \dots \}$ 
21   $(* \text{ Close invariant } *)$ 
22   $\{ \text{Thread}(\text{tid}, T_0) * \text{Proph}(p, \text{pvs}) * [\circ \{\text{tid}\}]^{\gamma_r} * \text{Tok} \}$ 
23  let  $v = \text{op } p \ r \ k$  in
24   $\{ \text{Thread}(\text{tid}, T_0) * [\circ \{\text{tid}\}]^{\gamma_r} * \text{Tok} * \text{Proph}(p, \text{pvs}') * (\text{pvs} = \text{prf} ++ \text{pvs}') \}$ 
25   $\{ \text{Thread}(\text{tid}, T_0) * [\circ \{\text{tid}\}]^{\gamma_r} * \text{Tok} * \text{Proph}(p, \text{pvs}') * \text{PastLin}(\text{op}, k, v_p, T_0) \}$ 
26  Resolve  $p$  to  $\text{END}(v)$ ;
27   $\{ \text{Thread}(\text{tid}, T_0) * [\circ \{\text{tid}\}]^{\gamma_r} * \text{Tok} * \text{Proph}(p, []) * (v_p = v) * \text{PastLin}(\text{op}, k, v_p, T_0) \}$ 
28   $(* \text{ Open invariant } *)$ 
29   $\{ \text{Thread}(\text{tid}, T_0) * [\circ \{\text{tid}\}]^{\gamma_r} * \text{Tok} * \text{PastLin}(\text{op}, k, v, T_0) * \text{CSS}(r, C_1) * \text{Inv}_{\text{help}}(H_1, T_1) * \dots \}$ 
30   $\{ \dots * \text{Tok} * [\circ \{\text{tid}\}]^{\gamma_r} * \text{PastLin}(\text{op}, k, v, T_0) * \text{State}(\text{op}, k, v, T_0, \Phi, \text{Tok}) \}$ 
31   $\{ \dots * \text{Tok} * \text{PastLin}(\text{op}, k, v, T_0) * \text{Done}(\text{op}, k, v, T_0, \Phi, \text{Tok}) \}$ 
32   $\{ \dots * \text{Tok} * \text{PastLin}(\text{op}, k, v, T_0) * (\Phi(v) \vee \text{Tok}) \}$ 
33   $\{ \dots * \Phi(v) * \text{PastLin}(\text{op}, k, v, T_0) * (\Phi(v) \vee \text{Tok}) \}$ 
34   $\{ \dots * \Phi(v) * \text{PastLin}(\text{op}, k, v, T_0) * \text{Done}(\text{op}, k, v, T_0, \Phi, \text{Tok}) \}$ 
35   $\{ \Phi(v) * \text{CSS}(r, C_1) * \text{Inv}_{\text{help}}(H_1, T_1) * \dots \}$ 
36   $(* \text{ Close invariant } *)$ 
37   $\{ \Phi(v) \}$ 
38   $v$ 
39   $\langle \text{res } C'. \text{CSS}(r, C') * \Psi_{\text{op}}(C, C', \text{res}) \rangle$ 

```

■ **Figure 16** Outline for the proof of the client-level specification for  $\text{op}$ .
